# Supplementary material for: Variance Reduction for Policy-Gradient Methods via Empirical Variance Minimization
Source: arXiv:2206.06827 source file (2022-06-15)
Supplement: Supplementary file 7 [file headerSupp.tex]

\usepackage{aistats2022}
% If your paper is accepted, change the options for the package
% aistats2022 as follows:
%
%\usepackage[accepted]{aistats2022}
%
% This option will print headings for the title of your paper and
% headings for the authors names, plus a copyright note at the end of
% the first column of the first page.

% If you set papersize explicitly, activate the following three lines:
%\special{papersize = 8.5in, 11in}
%\setlength{\pdfpageheight}{11in}
%\setlength{\pdfpagewidth}{8.5in}

% If you use natbib package, activate the following three lines:
\usepackage[round]{natbib}
\renewcommand{\bibname}{Supplementary References}
\renewcommand{\bibsection}{\section*{\bibname}}

% If you use BibTeX in apalike style, activate the following line:
%\bibliographystyle{apalike}

% Recommended, but optional, packages for figures and better typesetting:
\usepackage{microtype}
\usepackage{graphicx}
\usepackage{subfigure}
\usepackage{booktabs} % for professional tables

\usepackage{dsfont}
\usepackage{amsfonts,amsmath,amsthm,amssymb}
\usepackage{xargs}
\usepackage{thmtools,thm-restate}%appendix copying


%THEOREMS
\newcounter{asscnt}
\newtheorem{assum}[asscnt]{Assumption}
\newcounter{thcnt}
\newtheorem{theorem}[thcnt]{Theorem}
\newtheorem{proposition}[thcnt]{Proposition}
\newtheorem{lemma}[thcnt]{Lemma}


%COMMANDS
\DeclareMathOperator*{\argmax}{arg\,max}
\DeclareMathOperator*{\argmin}{arg\,min}
\newcommandx{\E}[1]{\mathds{E} \left[ #1 \right] }

\newcommandx{\Q}[1]{Q^{#1}}
\newcommandx{\V}[1]{V^{#1}}
\newcommandx{\norm}[2]{\left\Vert #1 \right\Vert_#2}



%\usepackage{natbib}
\bibliographystyle{plainnat}
\setcitestyle{authoryear} %Citation-related commands

\setcounter{thcnt}{2}
